# Supplementary material for: Learning Disentangled Semantic Spaces of Explanations via Invertible Neural Networks
Source: arXiv:2305.01713 source file (2024-06-11)
Supplement: Supplementary file 1 [file interpolation_examples_appendix.tex]

% \begin{table}[t]
% \begin{tcolorbox}[fontupper=\small, fontlower=\small]
% % \begin{enumerate}
% % \end{enumerate}
% \textcolor{blue}{an animal requires warmth in survival} \\
% 1. an animal requires warmth for survival \\
% 2. an animal requires oxygen for survival \\
% 3. some animals require oxygen for survival \\ 
% 4. humans sometimes require oxygen for survival \\
% 5. humans sometimes cause disease \\
% 6. humans cause disease \\
% 7. humans cause harm to other organisms \\
% 8. humans cause harm to themselves \\
% \textcolor{blue}{humans cause diseases}
% \end{tcolorbox}

% \caption{Interpolation examples.}
% \label{tab:interpol_examples_more}
% \end{table}
\begin{table}[ht!]
    % \resizebox{\textwidth}{15mm}{
% \begin{tikzpicture}
    \scriptsize
    \centering

    \begin{tabular}{p{7cm}p{7cm}}  \toprule
        \textcolor{blue}{an animal requires warmth in survival} \\ \hline
        1. an animal requires warmth for survival \\
        2. an animal requires oxygen for survival \\
        3. some animals require oxygen for survival \\ 
        4. humans sometimes require oxygen for survival \\
        5. humans sometimes cause disease \\
        6. humans cause disease \\
        7. humans cause harm to other organisms \\
        8. humans cause harm to themselves \\ \hline
        \textcolor{blue}{humans cause diseases} \\ \toprule
    \end{tabular}
    \caption{Interpolation.} 
    \label{tab:interpol_examples_more}
\end{table}
